# Supplementary material for: Analysis and Detection of Singing Techniques in Repertoires of J-POP Solo Singers
Source: arXiv:2210.17367 source file (2022-11-15)
Supplement: Supplementary file 1 [file appendix.tex]

% \documentclass{article}
% \usepackage[T1]{fontenc} % add special characters (e.g., umlaute)
% \usepackage[utf8]{inputenc} % set utf-8 as default input encoding
% \usepackage{ismir,amsmath,cite,url}
% \usepackage{graphicx}
% \usepackage{color}
% \newcommand{\yy}[1]{\textcolor{orange}{(YY: #1)}}

% \usepackage{todonotes}
% \usepackage{lineno}
% \linenumbers

% % Title. Please use IEEE-compliant title case when specifying the title here,
% % as it has implications for the copyright notice
% % ------
% \title{Appendix}
